# Supplementary material for: Characterizing Transaction-Reverting Statements in Ethereum Smart Contracts
Source: arXiv:2108.10799 source file (2021-09-01)
Supplement: Supplementary file 1 [file Appendix.tex]

\section{APPENDIX}

\subsection{Issues need to be solved}

\subsection{Mind Map}
Figure~\ref{mindmap} represents the mind map for the paper.
\begin{figure*}[htbp]
\centering 
\includegraphics[width=1\textwidth]{figures/mindmap.jpg} 
\caption{Mind Map for the paper} 
\label{mindmap} 
\end{figure*}
